# Supplementary material for: Freehand 2D Ultrasound Probe Calibration for Image Fusion with 3D MRI/CT
Source: arXiv:2303.07714 source file (2023-03-14)
Supplement: Supplementary file 1 [file appendix.tex]

\chapter{The first appendix}

\section{Algorithm}

\begin{itemize}
	\item The camera pose is estimated using MATLAB Camera Calibration Toolbox \cite 
\end{itemize}
